# Supplementary material for: Probing near-field EM fluctuations in superparamagnetic CoFeB with NV quantum dephasometry
Source: arXiv:2602.13341 source file (2026-02-12)
Supplement: Supplementary file 1 [file Supplementary.pdf]

# Supporting information

## Probing near-field EM fluctuations in superparamagnetic CoFeB with NV quantum dephasometry


Shoaib Mahmud[1,2,*], Wei Zhang[1,2,*], Pronoy Das[1,2], Angshuman Deka[2], Wenbo Sun[1,2], Zubin Jacob[1,2]

*Equal Contribution

[1]Elmore Family School of Electrical and Computer Engineering, Purdue University, West Lafayette, Indiana 47907, USA.
[2]Birck Nanotechnology Center, and Purdue Quantum Science and Engineering Institute, West Lafayette, Indiana 47907, USA.


# 1 Experimental setup

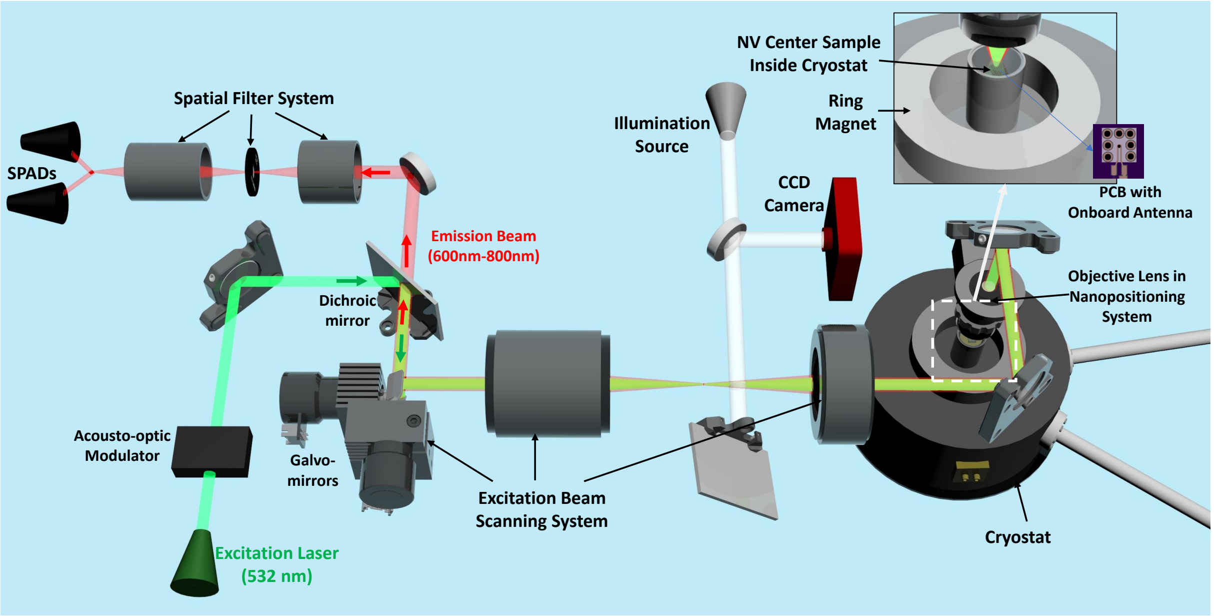


Figure S1: The experimental setup for quantum spectroscopy of the near-field electromagnetic (EM) fluctuations using NV centers in diamond. It is a home-built confocal setup capable of implementing different spectroscopy protocols.

We have conducted our measurements in a home-built confocal microscopy setup as shown in Fig. S1. The excitation source for the initialization and readout of nitrogen-vacancy (NV) centers is a 532 nm beam generated by a continuous-wave (CW) solid-state laser. For pulsed measurement, this beam is modulated by an acousto-optic modulator (AOM) controlled via a programmable TTL pulse generator. The laser is focused onto the NV center sample using an objective lens with a numerical aperture (NA) of 0.6. The objective lens has a maximum working distance of 4 mm and is collar-corrected for the 1 mm thick glass window of the cryostat. The lens focuses the green laser to a spot size of approximately 500 nm on the diamond sample. The diamond sample is mounted on the cold finger of the cryostat using a printed circuit board (PCB). A copper antenna on the PCB supplies an RF signal to the NV center sample. The RF signal is generated from a Keysight M8190A arbitrary waveform generator. The signal is amplified using a ZHL-16W-43-S+ high power amplifier. An external magnetic field is applied to the NV center sample by placing appropriate

magnets around the cryostat snout. Photoluminescence (PL) signals emitted from the diamond sample are collected with the same objective lens and passed through a dichroic mirror with a cutoff wavelength of 550 nm. The PL signal is detected using a pair of Micro Photon Devices SPADs. Higher spatial resolution is obtained using a pair of lenses with a pinhole aperture to collect only fluorescence from the objective's focal plane. The time-tagged PL signal is processed by a Hydraharp time-correlated single photon counting (TCSPC) device. This time-tagged signal is used to read the spin states of NV centers optically during different measurements.

# 2 Sample preparation and magnetic material deposition

The diamond plates used in this work are optical-grade diamond from Element Six. Upon receiving the diamond substrates, we processed the samples in Plasma-Therm Apex SLR inductively coupled etcher. The surface topography of the diamond substrates was characterized in the Park NX20 atomic force microscope (Fig. S2(a)), and the optical characterization of the NV-implanted substrates was conducted in the home-built confocal microscopy setup. Nitrogen ion implantation was performed by CuttingEdge Ions (Fig. S2(b)).

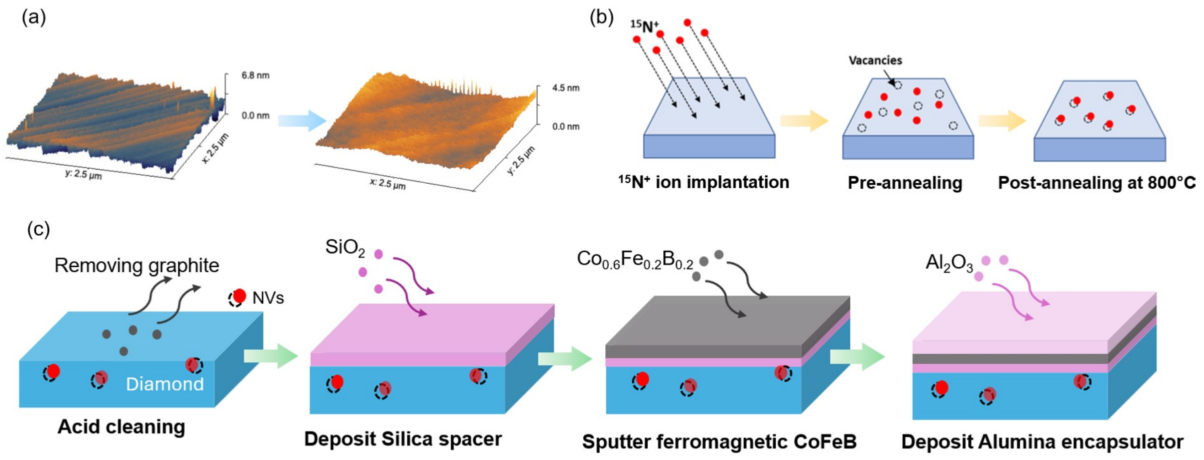


Figure S2: Diamond substrate processing and fabrication procedure. (a) Diamond surface topography profile showing improvement of surface roughness after plasma etching treatments. The surface profile is characterized using atomic force microscopy (AFM). (b) Nitrogen ion implantation and nitrogen vacancy formation in diamond substrate. (c) Deposition sequence to create a near-field interaction platform of magnetic CoFeB and NV centers.

In order to preserve the NV properties and to control the NV-material distance, we sputtered silica spacer directly on the surface of our diamond substrate (Fig. S2(c)). We deposited $SiO_2$ with thicknesses of 20, 30, 40 nm on the same substrate using a shadow mask placed on the diamond as shown in Fig. S3. The magnetic material was deposited onto the silica spacer on diamond using a stoichiometric target $Co_{60}Fe_{20}B_{20}$ in a physical vapor deposition (PVD) sputtering chamber with a base pressure of $10^{-6}$ Torr for magnetron sputtering. The CoFeB was deposited with a 30 W power in 15 sccm of Ar gas for 4 minutes, and was immediately encapsulated by 15 nm of Alumina sputtered in the same chamber. The magnetization measurements of the CoFeB-deposited diamond was performed in the Quantum Design MPMS-3 EverCool SQUID magnetometer using vibrating sample magnetometry (VSM). The VSM measurements was conducted both along the in-plane and normal direction to the diamond surface to characterize the magnetization of the as-deposited CoFeB in an applied magnetic field.

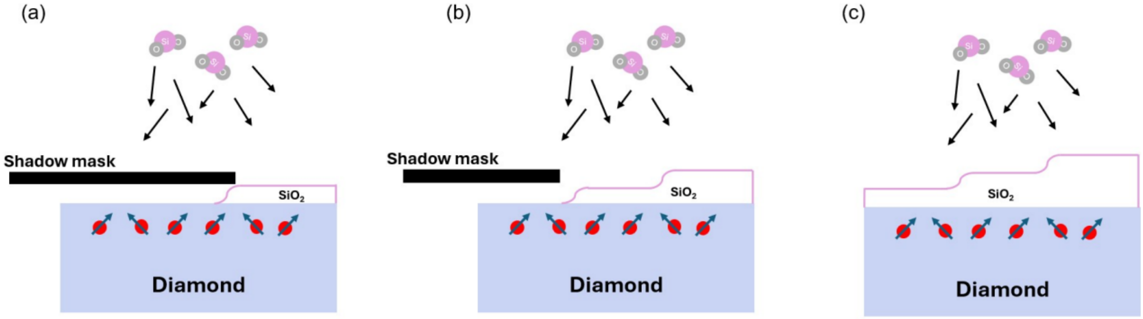


Figure S3: Fabrication method to create varying material-NV distance on the same diamond substrate. (a) A shadow mask was placed on the diamond substrate in the isotropic sputtering chamber to grow the first section of silica. (b) In the second sputtering, the mask was moved to cover one-third of the substrate. (c) The shadow mask was removed in the last sputtering run to create a three-step silica spacer of 20, 30, and 40 nm.

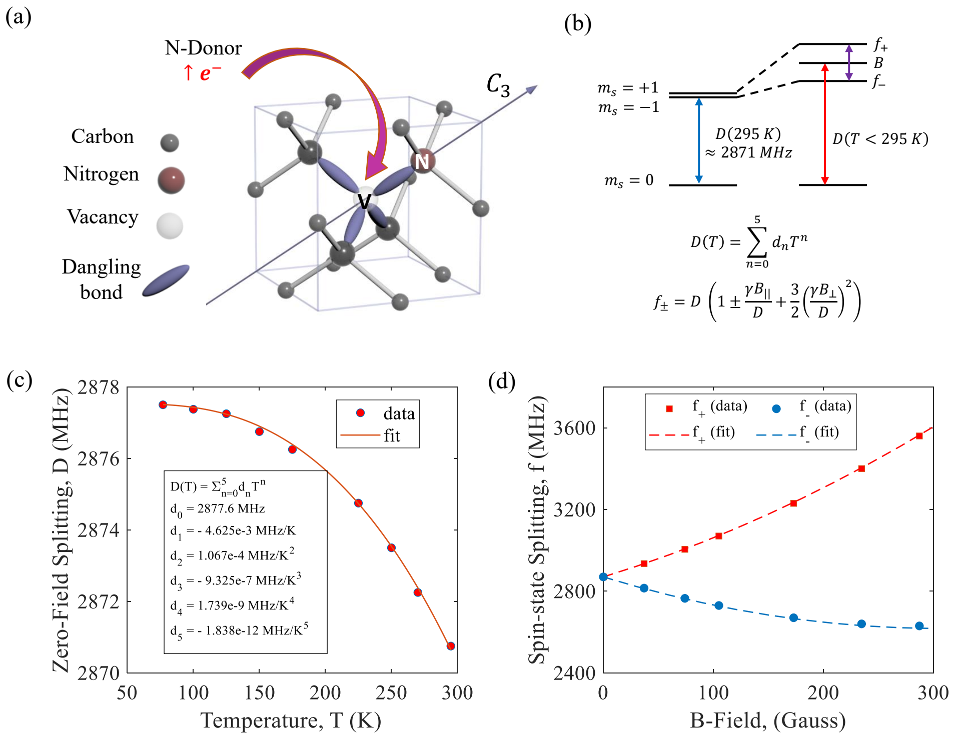


Figure S4: Temperature and magnetic field dependence of NV center ground-state energy levels. (a) Atomic structure of an NV center in diamond. (b) Electronic ground-state energy level structure of NV center spin qubit, illustrating the influence of temperature and magnetic field on the energy levels. (c) Temperature dependence of the zero-field splitting parameter. (d) Effect of an external magnetic field ($54.7^o$ with NV axis) on the spin sublevels of the NV center ground state.

## 3 Effect of temperature and magnetic field on NV energy levels

To implement the dephasometry protocol using NV center spin qubits in diamond, it is crucial to accurately determine their ground-state spin energy levels. These energy levels are sensitive to external parameters, particularly temperature and applied magnetic fields, which can induce shifts and splittings in the spin

sublevels [1, 2]. As a result, a detailed and precise characterization of how temperature and magnetic field affect the NV center's energy level structure is essential for high-fidelity quantum sensing and control. The atomic configuration of the NV defect, along with its electronic level structure, is shown in Fig. S4(a,b), highlighting the temperature and magnetic field dependencies. Fig. S4(c) presents our measured zero-field splitting parameter, $D(T)$, as a function of temperature $T$. The experimental data exhibit a non-linear trend and are well fitted using a fifth-order polynomial model, consistent with earlier reports [3]. Fig. S4(d) shows the effect of an externally applied magnetic field on the spin energy levels, where the fit corresponds to a magnetic field misalignment angle of $54.7^o$. These measurements form the basis for calibrating and applying the dephasometry protocol with high accuracy.

# 4 Setup of measurement protocols and parameters

Table S1 summarizes the key experimental parameters used for implementing the quantum relaxometry and dephasometry protocols to probe near-field EM fluctuations in CoFeB using NV centers in diamond. A $\pi$-pulse with a duration of approximately 20 ns is used to coherently manipulate the NV spin states. Optical initialization and readout are performed using a green laser with a spot diameter of around 500 nm, pulse duration of $\approx 5\ \mu s$, and power of approximately 500 $\mu$W. NV fluorescence is collected over an integration window of about 300 ns to ensure a sufficient signal-to-noise ratio. Each pulse sequence is repeated approximately $10^6$ times to accumulate statistically meaningful data. These parameters are optimized to achieve high measurement sensitivity while minimizing spin decoherence and thermal effects, as detailed in Ref. [4].

| Parameters | Values |
|---|---|
| $\pi-$pulse length | $\approx 20\ ns$ |
| Green laser spot diameter | $\approx 500\ nm$ |
| Green laser power | $\approx 500\ \mu W$ |
| Green laser pulse length | $\approx 5\ \mu s$ |
| NV photon count integration time | $\approx 300\ ns$ |
| Repetitions of the pulse sequence | $\approx 10^6$ |

Table S1: Parameters used for measuring the near-field EM fluctuations of CoFeB using NV centers.

# 5 Temperature dependence of the coherence times of NV centers in intrinsic and silver-deposited diamond

To underscore the unique temperature scaling of the coherence times of NV centers observed in the CoFeB system, we compare it to two other scenarios - intrinsic diamond and metallic silver. In intrinsic diamond, NV relaxation is predominantly governed by phonon-induced processes, which can be fitted by a three-parameter model as described in ref [5], as shown in Fig. S5(a). In contrast, the dephasing time $T_2$ is limited by quasi-static nuclear spin noise, which couples to NV centers via dipolar interactions and exhibits negligible temperature dependence, as seen in Fig. S5(b). In the case of a metallic silver layer, NV centers experience magnetic field noise arising from Johnson (thermal) noise of conduction electrons. The relaxation rate in this case scales as $1/T_1 \propto \sigma T$, where $\sigma$ is the electrical conductivity [6, 7]. However, as temperature increases, enhanced electron scattering reduces conductivity, partially canceling the thermal enhancement of Johnson noise. As a result, the net relaxation rate becomes nearly temperature-independent (Fig. S5(a)). Furthermore, the low-frequency component of this noise is too weak to substantially affect NV dephasing, leading to minimal temperature dependence in $T_2$ (Fig. S5(b)). In contrast, the CoFeB thin film shows a distinct and temperature-sensitive signature in both relaxation and dephasing times, due to its superparamagnetic fluctuations.

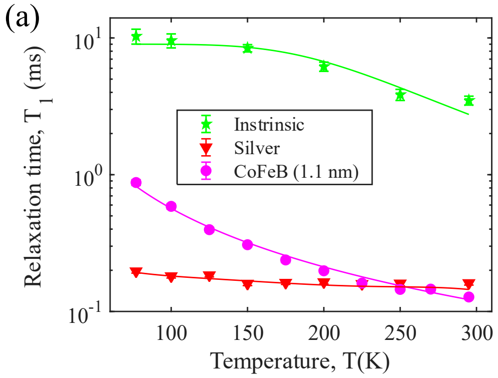


Figure S5: Comparison of the temperature scaling of the coherence times of NV centers in intrinsic and silver-deposited samples with that of CoFeB. (a) Temperature scaling of the relaxation time, $T_1$, of NV centers in instrinsic, silver and CoFeB-deposited samples. (b) Temperature scaling of the dephasing time, $T_2$, of NV centers in intrinsic, silver, and CoFeB-deposited samples.

# 6 Measurement of low-frequency noise spectrum using quantum dephasometry

Quantum dephasometry can be used to construct the frequency-dependent noise spectrum near materials. The pulse sequence used for this analysis is shown in Fig. S6(a). Here, the NV center spin qubits are first initialized into a superposition state using a $\pi/2$ pulse. A series of equally spaced $\pi$-pulses is then applied, followed by a final $\pi/2$ pulse for spin projection readout. The $\pi$-pulses modulate the influence of environmental noise on the NV center phase evolution. The resulting spin dynamics under this pulse sequence are illustrated in Fig. S6(a).

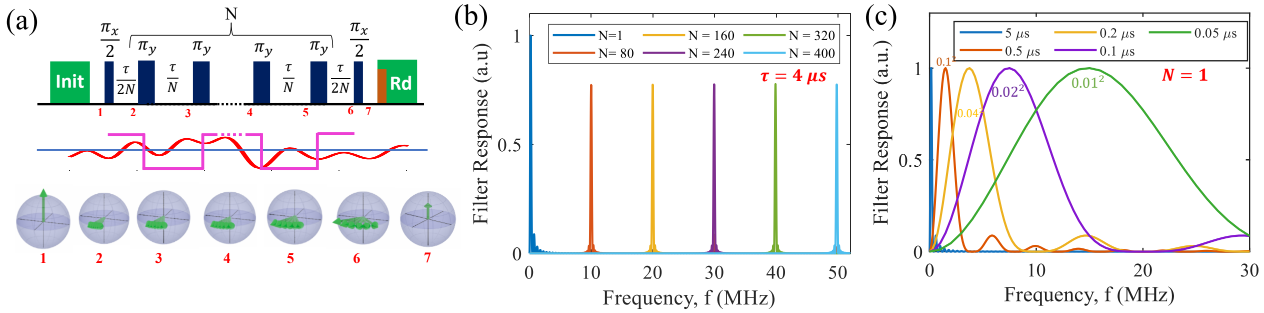


Figure S6: Low-frequency spectroscopic characterization of the CoFeB layer.(a) Quantum dephasometry using a dynamical decoupling pulse sequence. A schematic of the CPMG pulse sequence is shown, where an equidistant series of N of $\pi$-pulse (along the y-direction relative to the initial $\pi/2$-pulse) is applied to suppress noise components contributing to dephasing. The influence of the low-frequency noise on the phase of NV centers is illustrated through their evolution on the Bloch sphere. (b) Filter function for varying numbers (N) of $\pi$-pulses, a fixed $\tau = 4\mu s$. The central frequency of the filter shifts with N, allowing exploration of different spectral components. (c) Filter functions for $N = 1$ with varying $\tau$ durations. The filter function narrows in frequency as $\tau$ increases, enhancing sensitivity to specific noise bands.

The frequency components of the noise probed by this technique are determined by the corresponding noise filter functions, which depend on both the number of $\pi$-pulses and the spacing between them. Fig. S6(b) displays the filter functions for a total sequence duration of $\tau = 4$ $\mu s$, for various numbers of $\pi$-pulses. These filter functions are obtained via the Fourier transform of the phase modulation function depicted in Fig. S6(a). As shown, for a fixed $\tau$, the central frequency of the filter function shifts in the frequency domain

with fixed bandwidth as the number of $\pi$-pulses increases. In Fig. S6(c), we also consider the case where the number of $\pi$-pulses is fixed at $N = 1$, and $\tau$ is varied. The plot clearly shows that changing $\tau$ alters both the central frequency and the bandwidth of the filter function.

For our noise spectroscopy measurements, the total inter-pulse spacing, $\tau$ is kept constant while the number of $\pi$-pulses, N is varied. This procedure shifts the frequency response of the noise filter, as illustrated in Fig. S6(b). The coherence, $C(t)$, of the NV centers is measured at different positions of the noise filters, and the corresponding noise power spectral density at the filter center frequency is extracted using the relation [8]-

$$S(f) = -\frac{\pi \ln C(t)}{t}. \tag{1}$$

where, $t = \tau + Nt_\pi$ is the total evolution time of the dynamical decoupling sequence, with $\tau$ representing the wait time and $Nt_\pi$ the cumulative duration of the applied $\pi$-pulses.

# References


[1] Sunuk Choe et al. “Precise temperature sensing with nanoscale thermal sensors based on diamond NV centers”. In: *Current Applied Physics* 18.9 (2018), pp. 1066–1070.

[2] Jean Philippe Tetienne et al. “Magnetic-field-dependent photodynamics of single NV defects in diamond: an application to qualitative all-optical magnetic imaging”. In: *New Journal of Physics* 14.10 (2012), p. 103033.

[3] X-D Chen et al. “Temperature dependent energy level shifts of nitrogen-vacancy centers in diamond”. In: *Applied Physics Letters* 99.16 (2011).

[4] Shoaib Mahmud et al. “Quantum imaging of photonic spin texture in an OAM beam with NV centers in diamond”. In: *New Journal of Physics* 27.5 (2025), p. 054102.

[5] A Jarmola et al. “Temperature-and magnetic-field-dependent longitudinal spin relaxation in nitrogen-vacancy ensembles in diamond”. In: *Physical review letters* 108.19 (2012), p. 197601.

[6] S Kolkowitz et al. “Probing Johnson noise and ballistic transport in normal metals with a single-spin qubit”. In: *Science* 347.6226 (2015), pp. 1129–1132.

[7] Amila Ariyaratne et al. “Nanoscale electrical conductivity imaging using a nitrogen-vacancy center in diamond”. In: *Nature communications* 9.1 (2018), p. 2406.

[8] Nir Bar-Gill et al. “Suppression of spin-bath dynamics for improved coherence of multi-spin-qubit systems”. In: *Nature communications* 3.1 (2012), p. 858.
